# Supplementary material for: Deep Learning Collective Variables from Transition Path Ensemble
Source: arXiv:2303.01629 ancillary file (2023-03-02)
Supplement: Supplementary file 1 [file Supp_info.pdf]

# Supporting Information: Deep Learning Collective Variables from Transition Path Ensemble

Dhiman Ray,<sup>†</sup> Enrico Trizio,<sup>†,‡</sup> and Michele Parrinello<sup>\*,†</sup>

<sup>†</sup>*Atomistic Simulations, Italian Institute of Technology, Genoa, Via Enrico Melen 83, GE  
16153, Italy*

<sup>‡</sup>*Department of Materials Science, Università di Milano-Bicocca, Milano 20126, Italy*

E-mail: michele.parrinello@iit.it

# Computational Details

## Müller-Brown Potential

The TPI-Deep-TDA approach was first tested on the two dimensional Müller-Brown potential. All the simulation were performed using Langevin dynamics runs that used the Bussi-Parrinello algorithm<sup>1</sup> as implemented in the `ves_md_linearexpansion`. The damping constant in the Langevin equation was set to 10/time-unit. The time unit was defined arbitrarily and corresponds to 200 timesteps.<sup>2,3</sup> Natural units ( $k_B T = 1$ ) were used in all the calculations.

After having run unbiased simulations in the two metastable states for  $10^6$  time step. s We start by training a standard Deep-TDA CV.

From each trajectory a total 10000 points were randomly selected. Out of the total 20000 points, 14000 were used for training (with a batch size of 7000) and 6000 points were used for validation. As descriptors and input of the NN, we used the  $x$  and  $y$  coordinates. We used NN that had two hidden layers and a 2-6-4-1 architecture. The target mean and width of distributions corresponding to the two minima ( $A$  and  $B$ ) were  $\{\mu_A = -7.0, \mu_B = 7.0\}$  and  $\{\sigma_A = 0.5, \sigma_B = 0.5\}$ . The hyperparameters  $\alpha$  and  $\beta$  were chosen as 1 and 250. The Adam<sup>4</sup> optimizer was used with a learning rate of  $10^{-3}$  and a L<sub>2</sub> regularization term with a hyperparameter of  $10^{-5}$ .

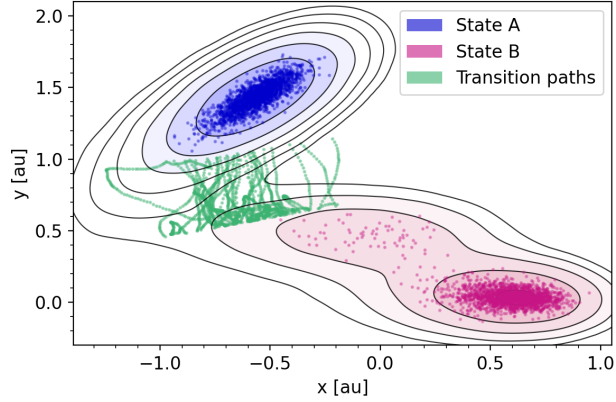

Figure S1: Scatter plot of the configurations for the training of deep learning collective variables for the Müller-Brown potential. The training data for the standard Deep-TDA CV is limited to the metastable states (blue and pink) while the in TPI-Deep-TDA also configurations from the transition path ensemble (green) are provided. The isolines of the true free energy surface are depicted in black.

To obtain data on the transition path ensemble (TPE), 30 OPES Flooding simulations were conducted using the Deep-TDA CV  $s$  with a filling factor  $\Delta E = 10 k_B T$  (TPE). Only those configurations whose  $s$  values where in the interval  $-3.5 < s < 2.0$  were considered to be part of the TPE.

To train the TPI-Deep-TDA CV, we used a total of 1714 configurations distributed roughly in equal number between the metastable states and the transition path ensemble configurations. The target mean and width of the Gaussians were selected as follows:

$\{\mu_A = -7.0, \mu_{TPE} = 0.0, \mu_B = 7.0\}$  and  $\{\sigma_A = 0.5, \sigma_{TPE} = 1.0, \sigma_B = 0.5\}$ . The NN training procedure was identical to what done in the Deep-TDA case except for the number of configurations used in the training and validation sets that were 1200 and 514 with a batch size of 600. A set of three OPES simulations were conducted on this new TPI-Deep-TDA CV with  $\Delta E = 20$  kJ/mol for  $2 \times 10^7$  time steps. A set of three OPES simulations were also performed with the initial Deep-TDA CV with identical parameters for comparison. During the simulations, half harmonic walls have been applied at  $s = \pm 8.5$  for the Deep-TDA CV, and  $s = \pm 8.0$  for the TPI-Deep-TDA CV to restrict the exploration of excessive-high energy conformations.

## Chignolin mini-protein

Next, we tested the usefulness of our new CV for the study of the protein folding problem; particularly, the folding and unfolding of the CLN025 mutant of Chignolin miniprotein. Long unbiased simulations performed using the specialized Anton supercomputer predicted the unfolding and folding timescale to be  $2.2 \pm 0.4 \mu\text{s}$  and  $0.6 \pm 0.1 \mu\text{s}$  respectively.<sup>5</sup> In the current work, we performed our simulations using the CHARMM22\* force field<sup>6</sup> used in Ref. 5, to make a direct comparison of our results with the unbiased data. The input configuration for each state was taken from our previous investigations.<sup>7,8</sup> The structure of the folded state is originally taken from the Protein Data Bank with PDB ID: 5AWL.<sup>9</sup> All simulations were performed in NVT ensemble at 340K with the Cuda-enabled version of GROMACS v2021.5<sup>10</sup> patched with the PLUMED v2.9.<sup>2,3</sup> The simulation conditions were the same as in Ref. 5. Detailed simulation parameters can be accessed from the input files provided with the manuscript (See Data Availability Statement).

To sample the transition path ensemble two different approaches were considered. In the first case, the standard Deep-TDA CV was used to conduct OPES-Flooding simulations, and configurations found in the successfully transiting trajectories were used in training. In the second case, we sampled transition path configurations from the OPES-Flooding trajectories generated in our previous work<sup>7</sup> using the Deep-TICA CV<sup>8</sup> trained on the long unbiased simulation.<sup>5</sup> In each case, two different sets of descriptors have been tested: (i) A relatively general descriptor set consisting of all 45 pairwise contacts between the 10  $C_\alpha$  atoms of the chignolin, and (ii) a more curated description set of 210 pairwise distances between selected heavy atoms, introduced by Bonati et al.<sup>8</sup> The details of the choice of the 210 distances are described in Ref. 8. In the rest of the manuscript, we refer to the CV constructed from the descriptor sets (i) and (ii) as the **contact CV** and the **distance CV**, respectively.

To train the CVs, 50 ns unbiased molecular dynamics simulations were performed in the folded and unfolded states. A harmonic wall was applied along the RMSD order parameter for the unfolded simulation to prevent a spontaneous folding of the protein. The structures were saved at 1 ps intervals, from which the contacts and the distance descriptors were extracted using `plumed driver`. The initial Deep-TDA CVs in both descriptors spaces were trained only on these two states. In both cases the mean and width of the target distributions were chosen as follows:  $\{\mu_A = -7.0, \mu_B = 7.0\}$  and  $\{\sigma_A = 0.2, \sigma_B = 0.2\}$ . For each state, 48000 structures were sampled. Out of the 96000 structures, 64000 were used for training with a batch size of 32000, and the rest, 32000 were used for validation. The NN architecture was 45-24-12-1 for the contact CV and 210-120-24-12-1 for the distance CV.

The Adam<sup>4</sup> optimizer was used with a learning rate and  $L_2$  regularization hyperparameters were chosen to be 0.001 and  $10^{-5}$  respectively.

Using the Deep-TDA CV  $s$ , OPES-Flooding simulations were performed starting from the folded state to sample the transition path ensemble. The barrier parameter  $\Delta E$  was set to 15 kJ/mol and excluded region boundary  $s_{exc}$  was -3.0. A total of 20 successful transitions were observed from which structures corresponding to  $-5.0 < s < 5.0$  were used for training the TPI-Deep-TDA CV based on  $C_\alpha$  contacts. For the distance CV, the transition region was chosen to be between -6 and 6 in the Deep-TDA CV space.

The TPI-Deep-TDA CV was trained following an identical protocol as the standard Deep-TDA CV except that an additional Gaussian was added in between the folded and the unfolded states. The target mean and width of this TS distribution was  $\mu_{TPE} = 0.0$  and  $\sigma_{TPE} = 1.5$ . A wider distribution was used for the transition state ensemble as these structures do not belong to a single metastable state, but include multiple configurations sampled during the entire pathway.

We contrasted the results obtained in OPES simulations that used Deep-TDA and TPI-Deep-TDA CVs. For each case, three independent simulations were propagated for 1  $\mu$ s. For all OPES simulations, a barrier parameter ( $\Delta E$ ) of 30 kJ/mol was used.

## Ligand receptor binding

We also test the applicability of our approach to the ligand-receptor binding problem, the central process in Computer-Aided Drug Discovery (CADD). To this end, we performed TPI-Deep-TDA simulations on a model host-guest complex involving the binding of the G2 guest to the tetramethylated octacid host (OAMe)<sup>11</sup> used in the Statistical Assessment of Modeling of Proteins and Ligands (SAMPL5) challenge.<sup>12</sup> A 13-dimensional descriptor set, identical to our previous work,<sup>13,14</sup> was used to describe the binding transition. The descriptors consisted in the linear distance between the binding pocket of the host and the center of mass of the guest ( $z$ ), the water coordination of 8 fixed virtual atoms placed along the path of ligand (un)binding, and water coordination of 4 heavy atoms of the G2 guest molecule. A detailed description of these descriptors can be found in Ref. 13. Similar to the study by Rizzi et al.,<sup>13</sup> the NN was trained only on the 12 water coordination numbers (with a 12-8-6-4-1 architecture). Subsequently, the two-dimensional CV space consisting of the  $z$  and the TPI-Deep-TDA order parameter was used for enhanced sampling. OPES simulations using the standard Deep-TDA CV, with the same descriptors set, have already been performed earlier,<sup>15</sup> so they are not repeated in the current work.

For training the TPI-Deep-TDA CV, first, 50 ns of unbiased MD simulations were performed in both bound and unbound states. To sample the transition path ensemble OPES-Flooding simulations were conducted starting from the bound configuration. Unlike the previous two examples, the ligand-receptor distance ( $z$ ) is used as the CV for the OPES-Flooding simulations, instead of the Deep-TDA CV. One reason for this choice is to showcase the versatility of our approach. Another reason is that this distance CV is the most obvious and straightforward description of the ligand binding process and is commonly used in the literature. A total of 13 successful transitions from the bound to the unbound state were sampled from which 170,000 data points were extracted that satisfied the criteria:  $0.8 \text{ nm} < z < 1.3 \text{ nm}$ . An equal number of points were sampled from the unbiased simula-

tions in each metastable state leading to a total of 510000 points as training data. Roughly 2/3rd of the points were used in training the NN CV while the rest is used for validation. The training set was divided into two equal-sized batches and an Adam<sup>4</sup> optimizer was used with a learning rate of 0.0025 and  $L_2$  regularization of  $10^{-5}$ . The target mean and width of the distributions were chosen as follows:  $\{\mu_A = -5.0, \mu_{TPE} = 0.0, \mu_B = 5.0\}$  and  $\{\sigma_A = 0.2, \sigma_{TPE} = 0.5, \sigma_B = 0.2\}$ . After constructing the NN CVs, three independent 200 ns long OPES simulations were performed with  $\Delta E = 40$  kJ/mol for each CV setup.

## Supplementary Results on Chignolin mini-protein

### Comparison between Contact and Distance based descriptors

We compared the performance of the TPI-Deep-TDA CVs that were based on contacts and distances as descriptors. Although the accuracy of the computed free energy difference is similar in both cases, using contact descriptors leads to a tighter confidence interval when compared to a TPI-Deep-TDA CV trained on distance descriptors (See Fig. S4). With the distance descriptors, the convergence of the free energy difference was only obtained within  $1 k_B T$  accuracy after  $\sim 600$  ns of with the standard Deep-TDA CV. Although the average free energy converged faster with the TPI-Deep-TDA CV, the variance of the result between independent run remains more than  $1 k_B T$  throughout the  $1 \mu s$  period. In comparison, the contact-CV performed better in terms of lower variance and better convergence.

### Effect of overlapping data in the training set

Another key observation from our study is that the overlap between the distributions of the metastable states and the transition path ensemble, during the training of the TPI-Deep-TDA CV, can lead to very poor performance, and the user should be careful to avoid any such overlap. For example, we also trained TPI-Deep-TDA CV from Deep-TICA simulation, we extracted transition path configurations from the OPES flooding study from Ref 7. Although the transition path data obtained from Deep-TDA-based flooding simulations were clearly distinct from the data corresponding to the folded and unfolded state, the Deep-TICA CV led to a significant overlap between the transition path ensemble and the unfolded state (Fig. S5). Such overlaps existed despite collecting the transition path points only from the barrier region of the FES along the Deep-TICA CV, a fact that can be deceiving. Due to this overlap, the unfolded state and the transition paths were not fully distinguished, which eventually led to almost  $5 k_B T$  disagreement between the predicted free energy from OPES simulation and unbiased reference (see Fig. S6). A slight improvement of the accuracy was observed, however, when the 210 distances were used as descriptors instead of the  $C_\alpha$  contacts, as the Deep-TICA CV was originally trained on these distance descriptors. Nevertheless, it is evident that an overlapping distribution of the transition state and any of the metastable states will lead to an overestimation of the free energy of that basin. So during the training of the TPI-Deep-TDA CV, the user needs to be careful to ensure there is no overlap between the structures sampled from the initial state, final state, and the transition path ensemble.

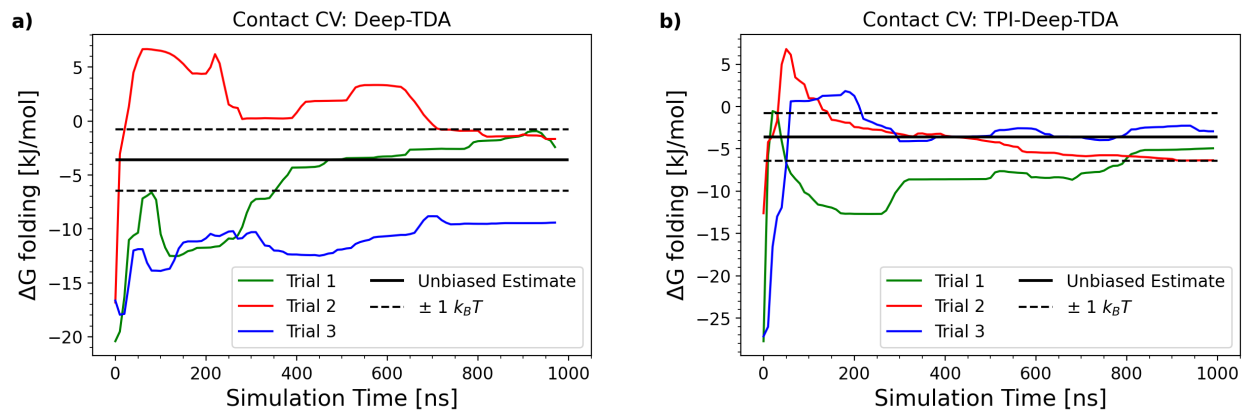

Figure S2: The convergence of the free energy difference between the folded and the unfolded states of Chignolin mini-protein using the Contact CV. The variance between the  $\Delta G$  values computed from independent trials is higher for the standard Deep-TDA CV (panel a) compared to the TPI-Deep-TDA CV (panel b).

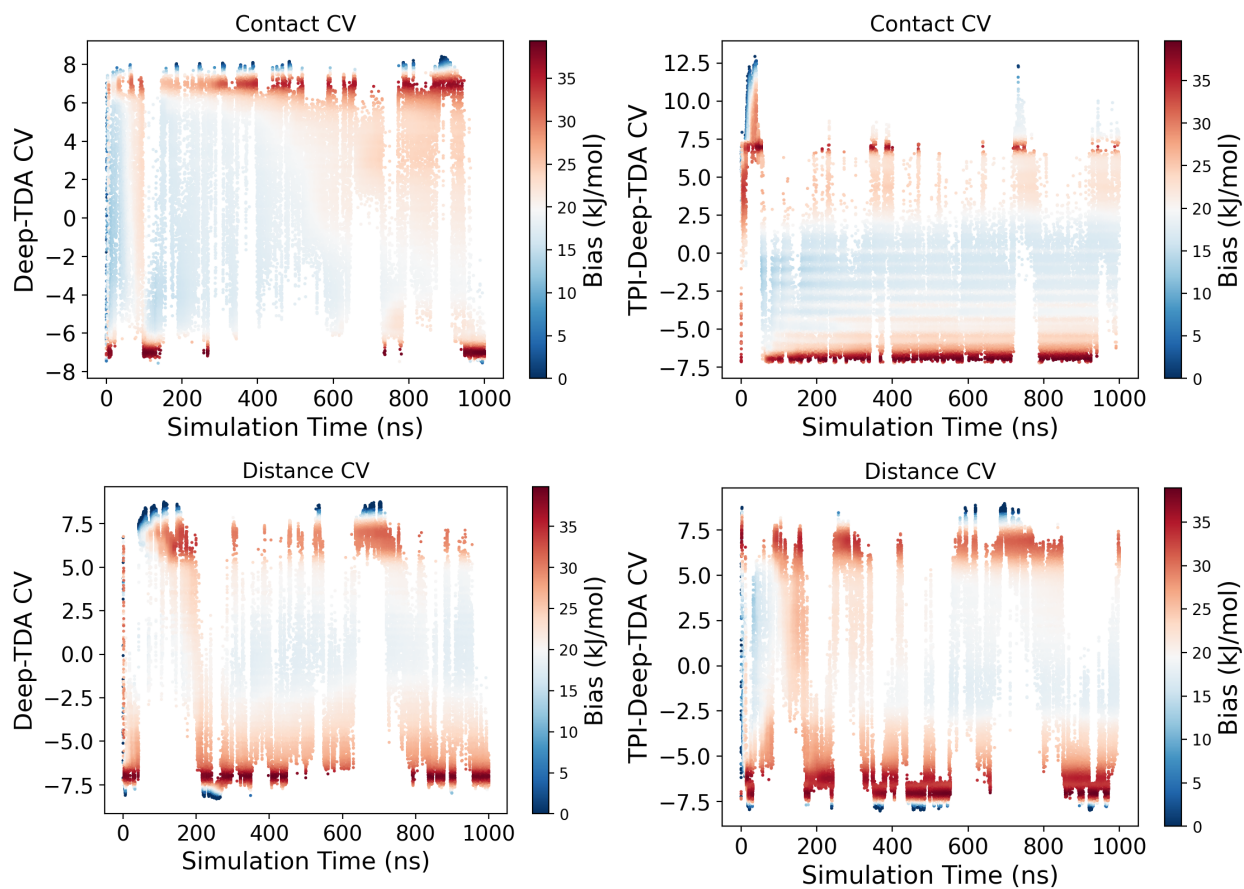

Figure S3: Representative time series of the standard Deep-TDA CV (left) and the TPI-Deep-TDA CV (right) for the contact-based (upper panel) and the distance-based (lower panel) descriptor set for the chignolin mini-protein.

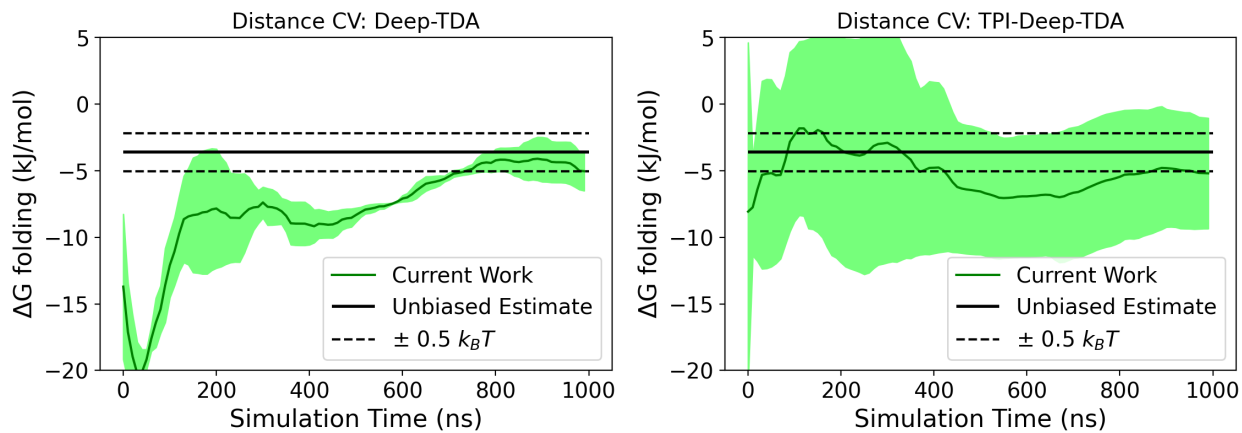

Figure S4: Convergence of the free energy of chignolin folding using OPES simulation for the standard Deep-TDA (left panel) and TPI-Deep-TDA (right panel) with the Distance CV. The green-shaded region is the standard deviation computed from three independent trajectories.

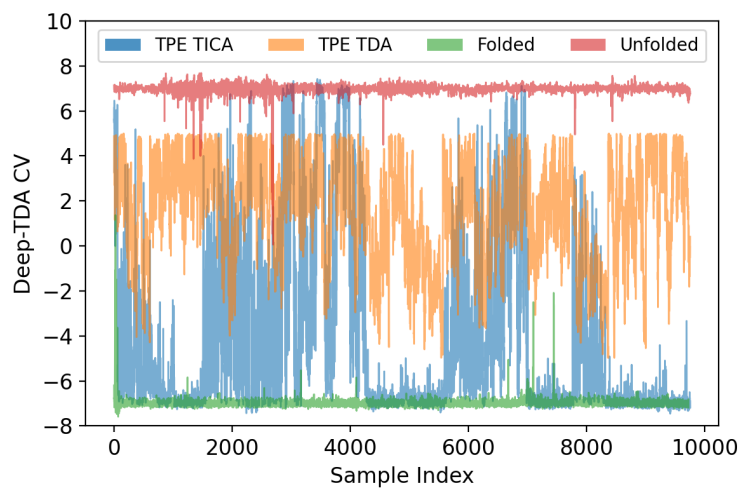

Figure S5: The data of the folded state, unfolded state and the transition path ensemble used for training the TPI-Deep-TDA CV, projected on the standard Deep-TDA CV with Contact descriptors. The transition path data sampled from OPES-Flooding simulation performed using the Deep-TDA CV (orange) does not overlap with the folded (green) or the unfolded (red) state. But the same obtained from OPES-Flooding simulations with Deep-TICA CV (blue) overlaps with both the metastable states. A CV trained in this manner leads to inaccurate predictions of the free energy profile.

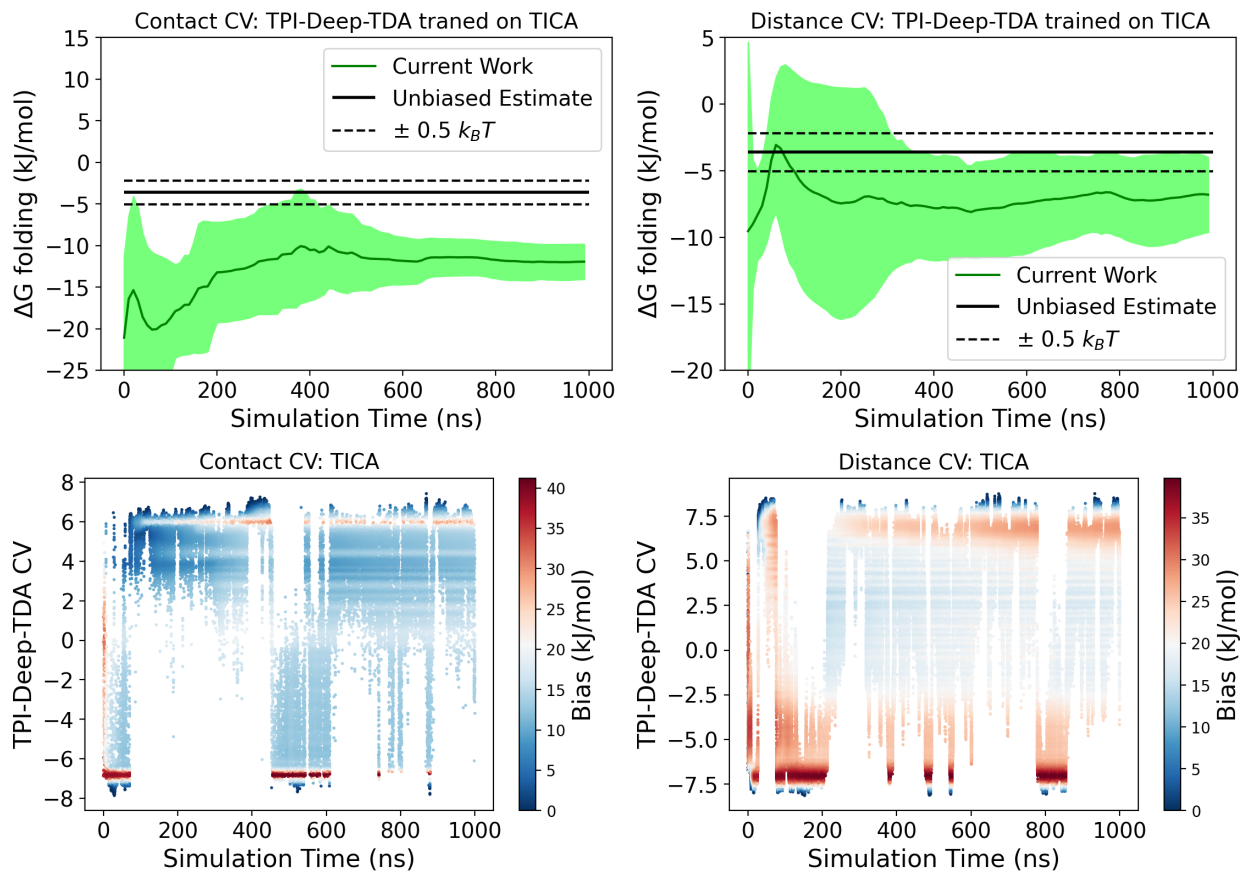

Figure S6: Upper panel: Convergence of the free energy of chignolin folding using OPES simulation for the TPI-Deep-TDA CV for which the transition paths were sampled from OPES flooding simulations with Deep-TICA CV. Lower panel: Representative time series of the CV during the OPES simulation.

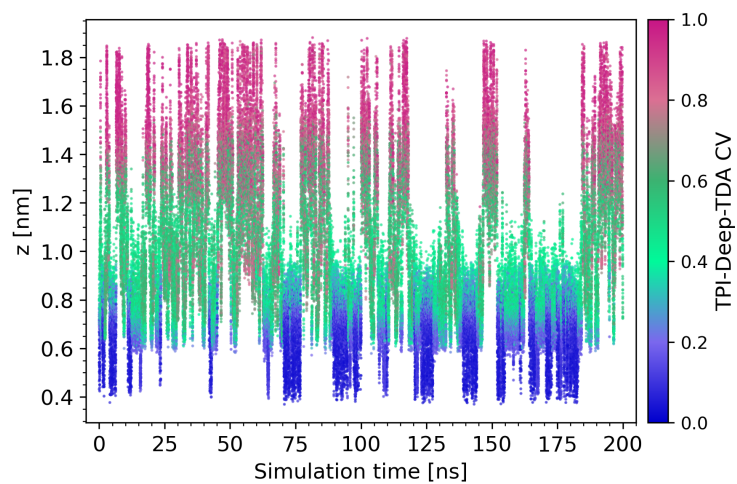

Figure S7: Time series of the  $z$  distance from the binding site during an OPES simulation using TPI-Deep-TDA and  $z$  as CVs. The color map depicts the value of the TPI-Deep-TDA CV.

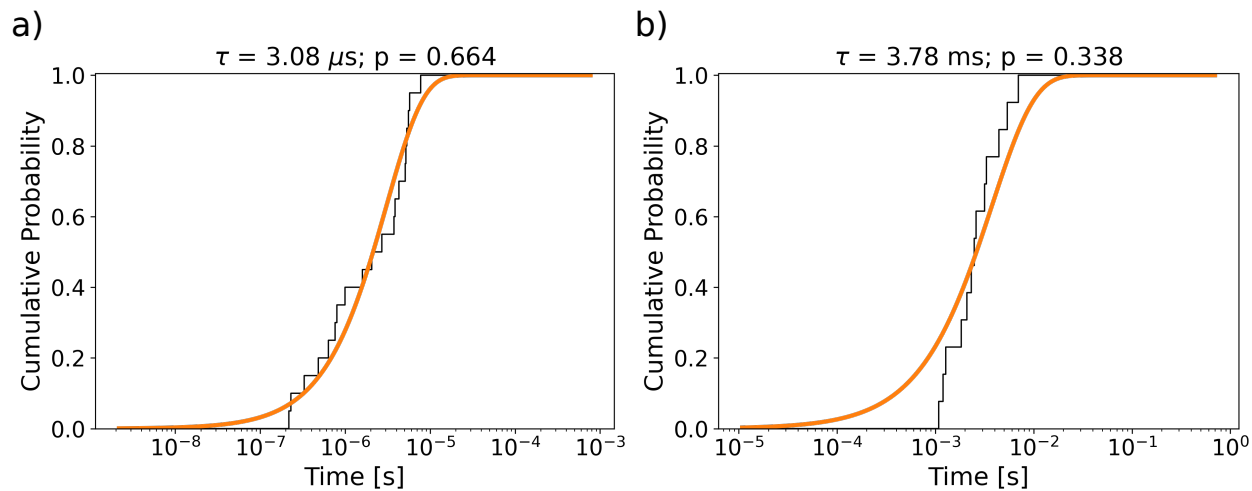

Figure S8: The quality of exponential fitting of the kinetic data of (a) the unfolding of chignolin and (b) the unbinding of G2 ligand from OAMe host. Detailed results are provided in main text.

## References

- (1) Bussi, G.; Parrinello, M. Accurate sampling using Langevin dynamics. *Physical Review E* **2007**, *75*, 056707.
- (2) Promoting transparency and reproducibility in enhanced molecular simulations. *Nature Methods* **2019**, *16*, 670–673.

- (3) Tribello, G. A.; Bonomi, M.; Branduardi, D.; Camilloni, C.; Bussi, G. PLUMED 2: New feathers for an old bird. *Computer Physics Communications* **2014**, *185*, 604–613.
- (4) Kingma, D. P.; Ba, J. Adam: A method for stochastic optimization. *3rd ICLR* **2014**,
- (5) Lindorff-Larsen, K.; Piana, S.; Dror, R. O.; Shaw, D. E. How fast-folding proteins fold. *Science* **2011**, *334*, 517–520.
- (6) Piana, S.; Lindorff-Larsen, K.; Shaw, D. E. How robust are protein folding simulations with respect to force field parameterization? *Biophysical Journal* **2011**, *100*, L47–L49.
- (7) Ray, D.; Ansari, N.; Rizzi, V.; Invernizzi, M.; Parrinello, M. Rare event kinetics from adaptive bias enhanced sampling. *Journal of Chemical Theory and Computation*
- (8) Bonati, L.; Piccini, G.; Parrinello, M. Deep learning the slow modes for rare events sampling. *Proceedings of the National Academy of Sciences* **2021**, *118*, e2113533118.
- (9) Honda, S.; Akiba, T.; Kato, Y. S.; Sawada, Y.; Sekijima, M.; Ishimura, M.; Ooishi, A.; Watanabe, H.; Odahara, T.; Harata, K. Crystal structure of a ten-amino acid protein. *Journal of the American Chemical Society* **2008**, *130*, 15327–15331.
- (10) Abraham, M. J.; Murtola, T.; Schulz, R.; Páll, S.; Smith, J. C.; Hess, B.; Lindahl, E. GROMACS: High performance molecular simulations through multi-level parallelism from laptops to supercomputers. *SoftwareX* **2015**, *1*, 19–25.
- (11) Gan, H.; Benjamin, C. J.; Gibb, B. C. Nonmonotonic assembly of a deep-cavity cavitand. *Journal of the American Chemical Society* **2011**, *133*, 4770–4773.
- (12) Yin, J.; Henriksen, N. M.; Slochower, D. R.; Shirts, M. R.; Chiu, M. W.; Mobley, D. L.; Gilson, M. K. Overview of the SAMPL5 host–guest challenge: Are we doing better? *Journal of Computer-Aided Molecular Design* **2017**, *31*, 1–19.
- (13) Rizzi, V.; Bonati, L.; Ansari, N.; Parrinello, M. The role of water in host-guest interaction. *Nature Communications* **2021**, *12*, 1–7.
- (14) Debnath, J.; Parrinello, M. Computing Rates and Understanding Unbinding Mechanisms in Host–Guest Systems. *Journal of Chemical Theory and Computation* **2022**, *18*, 1314–1319.
- (15) Trizio, E.; Parrinello, M. From enhanced sampling to reaction profiles. *The Journal of Physical Chemistry Letters* **2021**, *12*, 8621–8626.
